# Supplementary material for: Emergent fractals in hBN-encapsulated graphene based supermoir\'e structures and their experimental signatures
Source: arXiv:2502.19017 source file (2025-02-26)
Supplement: Supplementary file 1 [file supp_info.pdf]

# Emergent fractals in hBN-encapsulated graphene based supermoiré structures and their experimental signatures

Deepanshu Aggarwal, Rohit Narula, and Sankalpa Ghosh

*Department of Physics, Indian Institute of Technology Delhi, Hauz Khas, New Delhi 110016*

## I. DETAILS OF PARAMETER SPACE OF THE SUPERMOIRÉ SYSTEMS

The Table-I lists a number of linear mappings in the configuration space that include rotation between layers and dilation and were used in the main text.

Using the two vectors  $\{\mathbf{b}_1^{M(\ell'\ell)}, \mathbf{b}_2^{M(\ell'\ell)}\}$  defined in the main text, a  $2 \times 2$  matrix can be constructed as  $G_M = [\mathbf{b}_1^{M(\ell'\ell)} \ \mathbf{b}_2^{M(\ell'\ell)}]$ . The real-space moiré PV are then the columns of a matrix  $A_M$  such that

$$A_M = 2\pi G_M^{-1,T} = [\mathcal{I} - \mathcal{L}_{\ell'} \mathcal{L}_{\ell}^{-1}]^{-1,T} \mathcal{L}_{\ell} A \equiv \mathcal{L}_M A \quad (1)$$

In this work, we are particularly interested in generic trilayer SM systems, namely  $N = 3$ , and consider only the rotation of the top and bottom layers and keep the middle layer unrotated. Consequently, for the middle unrotated layer is  $A_2 = [\mathbf{a}_1^{(2)} \ \mathbf{a}_2^{(2)}]$  and for the top and bottom layers with  $\ell = 3, 1$  respectively, are  $A_{\ell} = (1 + \delta_{\ell 2}) \mathcal{R}(\theta_{\ell 2}) A_2$ , where  $\mathcal{R}$  is a two-dimensional rotation matrix, respective twist angles are  $\theta_{\ell 2}$ , and  $\delta_{\ell 2}$  is the lattice constant mismatch between the layer- $\ell$  and the middle layer, and is zero if the layers are same. Using Eq.1, the moiré wavelengths associated with individual moiré interfaces and their orientation *wrt* the attached coordinate system are respectively given by the individual moiré in each interface are the 2-norm of the column vectors in the matrix  $A_M^{(\ell,2)} = [\mathbf{a}_1^{M(\ell)} \ \mathbf{a}_2^{M(\ell)}]$  and can be written as

$$\lambda^M(\theta_{\ell 2}) = \frac{(1 + \delta_{\ell 2}) a}{\sqrt{2(1 + \delta_{\ell 2})[1 - \cos(\theta_{\ell 2})] + \delta_{\ell 2}^2}} \quad (2)$$

$$\tan(\Phi_{\ell 2}) = \frac{\sin(\theta_{\ell 2})}{1 + \delta_{\ell 2} - \cos(\theta_{\ell 2})} \quad (3)$$

where  $a = |\mathbf{a}_1^{(2)}| = |\mathbf{a}_2^{(2)}|$  is the lattice constant of middle layer.

### A. Supermoiré (SM) Harmonics

For a trilayer supermoiré systems under consideration, one can define SM harmonics labelled by integer pair  $(m, n)$ , such that the primitive reciprocal lattice vectors are given as the column vector of the matrix  $G_{SM}(m, n)$

$$G_{SM}(m, n) = \begin{bmatrix} m\mathbf{b}_{1x}^{M(1)} - n\mathbf{b}_{1x}^{M(2)} & m\mathbf{b}_{2x}^{M(1)} - n\mathbf{b}_{2x}^{M(2)} \\ m\mathbf{b}_{1y}^{M(1)} - n\mathbf{b}_{1y}^{M(2)} & m\mathbf{b}_{2y}^{M(1)} - n\mathbf{b}_{2y}^{M(2)} \end{bmatrix} \quad (4)$$

Here  $\mathbf{b}_i^{M(\ell'\ell)}$  are defined as the reciprocal lattice vectors of the constituent moiré-patterns in the main text. Unlike TBLG, where only lowest order harmonics dominate in the continuum limit, the dominant harmonic is twist angle dependent in such trilayer SM systems [1]. Corresponding primitive direct space lattice are the column vectors of the matrix  $A_{m,n}^{SM} = 2\pi G_{m,n}^{-1,T}$ . The 2-norm of the column vectors for each harmonic  $(m, n)$  of  $A_{m,n}$  can be defined as the associated the supermoiré length scale. However such supermoiré length scale not necessarily represents the actual periodicity of the resulting supermoiré system whose momentum space is infinite dimensional and lacks a BZ even in the continuum limit.

TABLE I. Linear mappings  $\mathcal{L}_1$ ,  $\mathcal{L}_2$  and  $\mathcal{L}_M$  for various cases.

|            | $\mathcal{L}_1$          | $\mathcal{L}_2$          | $\mathcal{L}_M$                      |
|------------|--------------------------|--------------------------|--------------------------------------|
| twist      | $\mathcal{R}(\theta/2)$  | $\mathcal{R}(-\theta/2)$ | $i\sigma_y \csc(\theta/2)/2$         |
| dilation   | $1 - \epsilon/2$         | $1 + \epsilon/2$         | $-1/\epsilon + \epsilon/4$           |
| pure shear | $1 - \epsilon\sigma_z/2$ | $1 + \epsilon\sigma_z/2$ | $(-1/\epsilon + \epsilon/4)\sigma_z$ |

Below, for generic SM systems where all constituent layers are hexagonal lattices, we list the real-space length scale for generic  $(m, n)$  with the different and same lattice mismatch of layer-1 and layer-3 *wrt* the middle layer, are

$$\lambda_{m,n}^{\text{SM}}(\theta_{12}, \theta_{32}, \delta_{12}, \delta_{32}) = a(\delta_{12} + 1)(\delta_{32} + 1) / \left[ (m - n)^2 (1 + \delta_{12})^2 (1 + \delta_{32})^2 \right. \quad (5a)$$

$$+ 2 \cos(\theta_{32})(mn - n^2)(1 + \delta_{32})(1 + \delta_{12})^2 + 2 \cos(\theta_{12})(mn - m^2)(1 + \delta_{12})(1 + \delta_{32})^2 \quad (5b)$$

$$\left. - m^2(1 + \delta_{12})^2 + n^2(1 + \delta_{32})^2 - 2mn \cos(\theta_{12} - \theta_{32})(1 + \delta_{12})(1 + \delta_{32}) \right]^{1/2} \quad (5c)$$

$$\lambda_{m,n}^{\text{SM}}(\theta_{12}, \theta_{32}, \delta_{12} = \delta_{32} = \delta) = a(\delta + 1) / \left[ (m - n)^2 (\delta^2 + 2\delta + 2) \right. \quad (5d)$$

$$\left. + 2(1 + \delta) [\cos(\theta_{12})(mn - m^2) + \cos(\theta_{32})(mn - n^2)] - 4mn \sin^2[(\theta_{12} - \theta_{32})/2] \right]^{1/2}$$

$$\lambda_{(m,m)}^{\text{SM}}(\theta_{12}, \theta_{32}, \delta_{12} = \delta_{32} = \delta) = \frac{a}{2|m \sin[(\theta_{12} - \theta_{32})/2]|} \quad (5e)$$

$$\lambda_{\text{SM}}^{(m,-m)} = \frac{a}{|m| \sqrt{2[3 + \cos(\theta_{12} - \theta_{32}) - 2(\cos(\theta_{12}) + \cos(\theta_{32}))]}} \quad (5f)$$

$$\lambda_{1,1}^{\text{SM}}(\theta_{12}, \theta_{32}, \delta_{12} = \delta_{32} = \delta) = \frac{a(\delta + 1)}{\sqrt{2(1 - \cos(\theta_{12} - \theta_{32}))}} \quad (5g)$$

$$\lambda_{(m,n)}^{\text{SM}}(\theta_{32} = -\theta_{12} = \theta, \delta_{12} = \delta_{32} = 0) = \frac{a}{2|\sin(\theta/2)| \sqrt{(m - n)^2 + 4mn \cos^2(\theta/2)}} \quad (5h)$$

$$\lambda_{(m,m)}^{\text{SM}}(\theta_{32} = -\theta_{12} = \theta, \delta_{12}, \delta_{32} = 0) = \frac{\lambda_{\text{M}}}{2|m \sin(\theta/2)|} \quad (5i)$$

where  $|\theta_{12}|, |\theta_{32}| \leq \pi/6$ .

## B. Diophantine Equation for commensurate SM structure

As mentioned in the main text for a trilateral SMS, the commensuration condition

$$\mathbf{a}_1^{\text{SM}} = n_1 \mathbf{a}_1^{\text{M}(1)} + n_2 \mathbf{a}_2^{\text{M}(1)} = n'_1 \mathbf{a}_1^{\text{M}(2)} + n'_2 \mathbf{a}_2^{\text{M}(2)} \quad (6)$$

The Eq.6, leads to the generic Diophantine equation in the natural lattice coordinates

$$\mathcal{L}_{12} A \begin{bmatrix} n_1 \\ n_2 \end{bmatrix} = \mathcal{L}_{32} A \begin{bmatrix} n'_1 \\ n'_2 \end{bmatrix} \quad (7)$$

which needs to be solved to give us the resulting commensurate structure. In words, it tells that there may exist a linear mapping  $\mathcal{L} = A^{-1} \mathcal{L}_{12}^{-1} \mathcal{L}_{32} A$  for the two moiré interfaces such that it maps a pair of integers  $(n'_1, n'_2)$  to  $(n_1, n_2)$ . For  $\theta_{12} = \theta_{32}$  and  $\delta_{12} = \delta_{32}$ , the linear mapping becomes an identity matrix. In the most generic trilateral case, the linear mapping  $\mathcal{L}$  becomes a function of four variables  $\theta_{12}, \theta_{32}, \delta_{12}, \delta_{32}$  such that the expanded matrix form of mapping on both sides of Eq.7 are

$$\mathcal{L}_{\ell 2} A = \begin{bmatrix} \frac{a(\delta_{\ell 2}^2 - \delta_{\ell 2} \cos(\theta_{\ell 2}) + 2\delta_{\ell 2} - \cos(\theta_{\ell 2}) + 1)}{\delta_{\ell 2}^2 - 2\delta_{\ell 2} \cos(\theta_{\ell 2}) + 2\delta_{\ell 2} - 2 \cos(\theta_{\ell 2}) + 2} & \frac{a(\delta_{\ell 2}^2 - 2\delta_{\ell 2} \sin(\theta_{\ell 2} + \frac{\pi}{6}) + 2\delta_{\ell 2} - 2 \sin(\theta_{\ell 2} + \frac{\pi}{6}) + 1)}{2(\delta_{\ell 2}^2 - 2\delta_{\ell 2} \cos(\theta_{\ell 2}) + 2\delta_{\ell 2} - 2 \cos(\theta_{\ell 2}) + 2)} \\ \frac{a(\delta_{\ell 2} + 1) \sin(\theta_{\ell 2})}{\delta_{\ell 2}^2 - 2\delta_{\ell 2} \cos(\theta_{\ell 2}) + 2\delta_{\ell 2} - 2 \cos(\theta_{\ell 2}) + 2} & \frac{a(\sqrt{3}\delta_{\ell 2}^2 - 2\delta_{\ell 2} \cos(\theta_{\ell 2} + \frac{\pi}{6}) + 2\sqrt{3}\delta_{\ell 2} - 2 \cos(\theta_{\ell 2} + \frac{\pi}{6}) + \sqrt{3})}{2(\delta_{\ell 2}^2 - 2\delta_{\ell 2} \cos(\theta_{\ell 2}) + 2\delta_{\ell 2} - 2 \cos(\theta_{\ell 2}) + 2)} \end{bmatrix} \quad (8)$$

In order to ensure that the two moiré makes a commensurate angle with each other, we first find the relation between the misorientation or twist angle  $(\theta)$  between a hBN and graphene, namely,

$$\theta = \sin^{-1}[(1 + \delta) \sin(\phi)] - \phi \quad (9)$$

where  $\delta$  is the lattice mismatch and  $\phi$  is the orientation of the moiré-pattern *wrt* the attached coordinate system. One needs to set the angles  $\theta_{12}$  and  $\theta_{32}$  in top and bottom interfaces, such that the moiré-patterns in the two interfaces make a commensurate angle between them. For these two angles, we evaluate the moiré wavelength and the misorientation  $\Phi_{\ell e}$  of the upper and lower surface using the expression (2) and (3). The difference between these two angles must match with the commensurate angle  $\theta_r$  calculated from the Diophantine equation.

## II. THE DERIVATION OF EFFECTIVE HAMILTONIAN $H_{\text{eff}}^{(1,2)}$ FOR HBN-GRAPHENE(BLG)-HBN SUPERMOIRÉ SYSTEM

To construct an effective low-energy theory we note that the chemical potentials of boron and nitrogen atoms in hBN are  $\mu_B = 3.34\text{eV}$  and  $\mu_N = -1.4\text{eV}$  [2], and in a perturbatively obtained low-energy effective Hamiltonian of graphene (G)-hBN, this difference appears in the denominator. Therefore, the low-energy spectrum in G-hBN is dominated by the electronic states of the graphene layer(s). Using the same argument for trilayer hBN-G(BLG)-hBN, the low-energy electronic spectrum is also dominated by the states of the middle graphene layer. To obtain the low-energy description, we explicitly write the effective Hamiltonian in hBN-G-hBN ( $H^{(1)}$ ) and hBN-BLG-hBN ( $H^{(2)}$ ) respectively in the direct product Hilbert spaces of the constituent layers that are  $\mathcal{S}_{\text{hBN}}^{(1)} \otimes \mathcal{S}_{\text{G}}^{(2)} \otimes \mathcal{S}_{\text{hBN}}^{(3)}$ , and  $\mathcal{S}_{\text{hBN}}^{(1)} \otimes \mathcal{S}_{\text{G}}^{(2)} \otimes \mathcal{S}_{\text{G}}^{(3)} \otimes \mathcal{S}_{\text{hBN}}^{(4)}$ . Consequently the Hamiltonians of these trilayer supermoiré systems can also be written in the basis set of six and eight states that corresponds to six and eight sublattices in the three and four layers, namely  $\{\psi_{A1}, \psi_{B1}, \psi_{A2}, \psi_{B2}, \psi_{A3}, \psi_{B3}\}$ , and  $\{\psi_{A1}, \psi_{B1}, \psi_{A2}, \psi_{B2}, \psi_{A3}, \psi_{B3}, \psi_{A4}, \psi_{B4}\}$ .

$$H^{(1)}(\mathbf{r}) = \begin{bmatrix} h_{\text{hBN},\xi}^{(1)}(\mathbf{r}) & V_{\xi}^{(12)}(\mathbf{r}) & 0 \\ V_{\xi}^{(12)\dagger}(\mathbf{r}) & h_{\text{G},\xi}^{(2)}(\mathbf{r}) & V_{\xi}^{(23)}(\mathbf{r}) \\ 0 & V_{\xi}^{(23)\dagger}(\mathbf{r}) & h_{\text{hBN},\xi}^{(3)}(\mathbf{r}) \end{bmatrix}; \quad (10)$$

$$H^{(2)}(\mathbf{r}) = \begin{bmatrix} h_{\text{hBN},\xi}^{(1)}(\mathbf{r}) & V_{\xi}^{(12)}(\mathbf{r}) & 0 & 0 \\ V_{\xi}^{(12)\dagger}(\mathbf{r}) & h_{\text{G},\xi}^{(2)}(\mathbf{r}) & \tilde{V}_{\xi}^{(23)} & 0 \\ 0 & \tilde{V}_{\xi}^{(23)\dagger} & h_{\text{G},\xi}^{(3)}(\mathbf{r}) & V_{\xi}^{(34)}(\mathbf{r}) \\ 0 & 0 & V_{\xi}^{(34)\dagger}(\mathbf{r}) & h_{\text{hBN},\xi}^{(4)}(\mathbf{r}) \end{bmatrix} \quad (11)$$

Here the  $h^i$ 's in the main diagonal of  $H^{(1,2)}$  describe the intralayer Hamiltonian of each individual layer in both structures in the valley  $\xi$ , the off-diagonal terms  $V_{\xi}^{(ij)}(\mathbf{r})$  are the interlayer hopping matrices between layers- $i$  and  $j$  that are moiré periodic, the constant potential  $\tilde{V}_{\xi}^{(23)}$  is the interlayer potential in BLG,  $v_F$  is the Fermi velocity in graphene, and  $v_{\text{BN}}$  is the Fermi velocity in hBN. The explicit form of these expressions is as follows:

$$h_{\text{hBN},\xi}^{(1)}(\mathbf{r}) = -i\hbar v_{\text{BN}} \boldsymbol{\sigma}_{\xi}^{(1)} \cdot \nabla + m v_{\text{G}}^2 \sigma_z + V \quad (12a)$$

$$h_{\text{G},\xi}^{(2)}(\mathbf{r}) = -i\hbar v_F \boldsymbol{\sigma}_{\xi}^{(2)} \cdot \nabla \quad (12b)$$

$$h_{\text{G},\xi}^{(2,3)}(\mathbf{r}) = -i\hbar v_F \boldsymbol{\sigma}_{\xi}^{(2,3)} \cdot \nabla + \text{diag}(\epsilon_{A2,A3}, \epsilon_{B2,B3}) \quad (12c)$$

$$h_{\text{hBN},\xi}^{(3,4)}(\mathbf{r}) = -i\hbar v_{\text{BN}} \boldsymbol{\sigma}_{\xi}^{(3)} \cdot \nabla + m v_{\text{G}}^2 \sigma_z - V \quad (12d)$$

$$V_{\xi}^{(\ell\ell')}(\mathbf{r}) = \frac{\gamma}{3} \sum_{n=1}^3 e^{i\delta \mathbf{K}_{n,\xi}^{(\ell\ell')} \cdot \mathbf{r}} \begin{pmatrix} 1 & e^{i\xi\phi_n} \\ e^{-i\xi\phi_n} & 1 \end{pmatrix} \quad (12e)$$

$$\tilde{V}_{\xi}^{(23)} = \begin{bmatrix} -v_4\pi & v_3\pi^\dagger \\ \gamma_1 & -v_4\pi \end{bmatrix} \quad (12f)$$

In the above expressions, the Dirac mass  $m$  in 12a and 12a occurs due to the difference between the onsite-potentials of Boron and Nitrogen in hBN,  $V$  is the external bias-voltage that can be due to a perpendicular uniform electric field, and  $\delta \mathbf{K}_n^\xi$  is the difference vector between two closest valley  $\xi$  in graphene and hBN. The second-order diagonal matrix in 12c that appears in  $H^{(2)}$  is due to the on-site potentials that result from the dimer-formation in Bernal-stacked BLG [3, 4]. In the basis set of Bloch states corresponding to six sublattices in graphene and the two hBN layers, in the second quantised notation, the Hamiltonian of this system reads  $H = \sum_{\xi} H_{\xi}$  where  $H_{\xi}$  is

$$H_{\xi} = \int d^2\mathbf{r} \hat{\Psi}_{\xi}^{\dagger}(\mathbf{r}) \begin{bmatrix} H_{\text{hBN},\xi} & V_{\xi}^{(12)}(\mathbf{r}) & 0 \\ V_{\xi}^{(12)\dagger}(\mathbf{r}) & H_{\text{G},\xi} & V_{\xi}^{(23)}(\mathbf{r}) \\ 0 & V_{\xi}^{(23)\dagger}(\mathbf{r}) & H_{\text{hBN},\xi}(\mathbf{r}) \end{bmatrix} \hat{\Psi}_{\xi}(\mathbf{r}) \quad (13)$$

where  $\xi = \pm 1$  is the valley index and the six-component field operator is  $\hat{\Psi}_{\xi}(\mathbf{r}) = (\psi_{\text{hBN},\xi}(\mathbf{r}) \ \psi_{\text{G},\xi}(\mathbf{r}) \ \psi_{\text{hBN},\xi}(\mathbf{r}))^T$ .

The single particle states can be obtained by diagonalising the  $6 \times 6$  Hamiltonian  $H(\mathbf{r})$  in Eq.A1, namely,

$$\begin{bmatrix} H_{\text{hBN},\xi} & V_{\xi}^{(12)}(\mathbf{r}) & 0 \\ V_{\xi}^{(12),\dagger}(\mathbf{r}) & H_{\text{G},\xi} & V_{\xi}^{(32)\dagger}(\mathbf{r}) \\ 0 & V_{\xi}^{(32)}(\mathbf{r}) & H_{\text{int}}^{\dagger}(\mathbf{r}) \end{bmatrix} \begin{bmatrix} \phi_1(\mathbf{r}) \\ \phi_2(\mathbf{r}) \\ \phi_3(\mathbf{r}) \end{bmatrix} = E \begin{bmatrix} \phi_1(\mathbf{r}) \\ \phi_2(\mathbf{r}) \\ \phi_3(\mathbf{r}) \end{bmatrix} \quad (14)$$

The above matrix equation leads to three coupled equations in  $\phi_1, \phi_2$  and  $\phi_3$  and consequently, two out of the three equations can be substituted for  $\phi_1$  and  $\phi_3$  to obtain a final equation in  $\phi_2$ , that is, in general, can be written as  $H_{\text{eff},\xi}(\mathbf{r}, E)\phi_2(\mathbf{r}) = 0$ , where the effective Hamiltonian operator  $H_{\text{eff},\xi}(\mathbf{r}, E)$  is given by

$$H_{\text{eff},\xi}(\mathbf{r}, E) = H_{\text{G},\xi}^{(2)}(\mathbf{r}) + V_{\xi}^{(12)\dagger}(\mathbf{r}) \left(E - H_{\text{hBN},\xi}^{(1)}\right)^{-1} V_{\xi}^{(12)}(\mathbf{r}) + V_{\xi}^{(32)\dagger}(\mathbf{r}) \left(E - H_{\text{hBN},\xi}^{(3)}\right)^{-1} V_{\xi}^{(32)}(\mathbf{r}) \quad (15)$$

The two terms, other than the graphene Hamiltonian, are translationally invariant with the moiré-pattern lattice vectors of respective interfaces. The inverse operators being the Green's function, we can introduce effective potentials

$$\tilde{U}^{(12)}(\mathbf{r}, E) = V_{\xi}^{(12)\dagger}(\mathbf{r}) \hat{G}^{(1)}(\mathbf{r}, E) V_{\xi}^{(12)}(\mathbf{r}) \quad (16a)$$

$$\tilde{U}^{(32)}(\mathbf{r}, E) = V_{\xi}^{(32)\dagger}(\mathbf{r}) \hat{G}^{(3)}(\mathbf{r}, E) V_{\xi}^{(32)}(\mathbf{r}) \quad (16b)$$

where  $\hat{G}^{(\ell)}(\mathbf{r}, E) \equiv \hat{G}^{(\ell)}(\mathbf{r}, \mathbf{r}; E) = \left(E - H_{\text{hBN},\xi}^{(\ell)}\right)^{-1}$  is the on-site single-particle Green's function at a particular spatial point  $\mathbf{r}$  and energy  $E$ . This readily gives the single particle Hamiltonian (15) at a given energy  $E$ .

### A. Evaluation of the Green's function

The Green's function that appeared in the expressions 16 can be evaluated by noting that

$$\hat{G}^{(\ell),-1}(\mathbf{r}, E) = E - H_{\text{hBN},\xi}^{(\ell)}(\mathbf{r}) \quad (17)$$

where  $H_{\text{hBN},\xi}^{(\ell)} = [-i\hbar v_{\text{BN}} \boldsymbol{\sigma} \cdot \nabla + mv^2 \sigma_z + V]$  such that

$$\hat{G}^{-1}(\mathbf{r}, E) \begin{pmatrix} u_1(\mathbf{k}) \\ u_2(\mathbf{k}) \end{pmatrix} e^{i\mathbf{k} \cdot \mathbf{r}} = \epsilon \begin{pmatrix} u_1(\mathbf{k}) \\ u_2(\mathbf{k}) \end{pmatrix} e^{i\mathbf{k} \cdot \mathbf{r}} \quad (18)$$

It is now straightforward to see that in the momentum representation, we can write  $\hat{G}^{-1}(\mathbf{r}, E)$  as

$$G^{-1}(k, E) = G_0^{-1}(E) - \tilde{V}(k) \quad (19)$$

This gives us straightforwardly the perturbative expansion for the Green's function as

$$\begin{aligned} G(k, E) &= G_0(E) + G_0(E) \tilde{V}(k) G(k, E) \\ &= G_0(E) + G_0(E) \tilde{V}(k) G_0(E) + G_0(E) \tilde{V}(k) G_0(E) \tilde{V}(k) G_0(E) + \dots \end{aligned} \quad (20)$$

where  $\tilde{V}(k)$  and  $G_0(E)$  are

$$\tilde{V}(k) = \begin{pmatrix} 0 & \hbar v_{\text{BN}}(k_x - ik_y) \\ \hbar v_{\text{BN}}(k_x + ik_y) & 0 \end{pmatrix} \quad \text{and} \quad G_0(E) = \frac{1}{E + mv^2 - V} \begin{pmatrix} \eta & 0 \\ 0 & 1 \end{pmatrix} \quad (21)$$

with  $\eta = (E - mv^2 - V)/(E + mv^2 - V)$  as a dimensionless parameter.

In the above equation,  $\eta \hbar v_{\text{BN}} \ll (E + mv^2)^2$  for low-energies  $|E| \ll mv^2$ , therefore, the  $k$ -dependent terms in the single-particle propagator are neglected. This will finally lead to the effective potentials  $U$  in the two-interfaces as

$$U^{(21)}(\mathbf{r}) = V^{(12),\dagger}(\mathbf{r}) h_{\text{hBN}}^{(1),-1} V^{(12)}(\mathbf{r}) \quad (22a)$$

$$U^{(23)}(\mathbf{r}) = V^{(32),\dagger}(\mathbf{r}) h_{\text{hBN}}^{(3),-1} V^{(32)}(\mathbf{r}) \quad (22b)$$

and appeared in the Hamiltonian  $H_{\text{eff}}^{(1)}$  in the main text. The explicit form of the potentials and the various parameters are taken from the Refs.[5, 6]

$$U^{(2\ell)}(\mathbf{r}) = \left( w_0 + u_0 g_1^{(2\ell)}(\mathbf{r}) + \tilde{u}_0 g_2^{(2\ell)}(\mathbf{r}) \right) \sigma_0 + \left( \tilde{w}_3 + u_3 g_2^{(2\ell)}(\mathbf{r}) + \tilde{u}_3 g_1^{(2\ell)}(\mathbf{r}) \right) \sigma_3 \\ + \left[ \hat{z} \times \frac{1}{|G|^{(2\ell)}} \left( u_{\perp} \nabla g_2^{(2\ell)}(\mathbf{r}) + \tilde{u}_{\perp} \nabla g_1^{(2\ell)}(\mathbf{r}) \right) \right] \cdot \boldsymbol{\sigma} + \frac{1}{|G|^{(2\ell)}} \left( u_{\parallel} \nabla g_2^{(2\ell)}(\mathbf{r}) + \tilde{u}_{\parallel} \nabla g_1^{(2\ell)}(\mathbf{r}) \right) \cdot \boldsymbol{\sigma} \quad (23)$$

where the spatially dependent terms  $g(\mathbf{r})$  which make  $U^{(2\ell)}(\mathbf{r})$  moiré-periodic, are given by

$$g_1^{(2\ell)}(\mathbf{r}) = 2 \sum_{j=1}^3 \cos(\mathbf{G}_j^{(2\ell)} \cdot \mathbf{r}) \quad (24)$$

$$g_2^{(2\ell)}(\mathbf{r}) = -2 \sum_{j=1}^3 \sin(\mathbf{G}_j^{(2\ell)} \cdot \mathbf{r}) \quad (25)$$

For the moiré reciprocal lattice vectors, the superscript  $2\ell$  indicates the layers involved, and it's numbered according to Fig.2 of the main text, with  $\ell = 1, 3$  of the hBN layers. The subscript  $j$  runs from 1 to 3 numbers where the vector  $\mathbf{G}_3^{l1'} = -\mathbf{G}_1^{l1'} - \mathbf{G}_2^{l1'}$ .

Similar to the trilayer hBN-G-hBN case, for hBN-BLG-hBN, the effects of the top and bottom hBN layers are considered equivalent to substrate moiré-periodic potentials. In doing so the eight-component Hamiltonian in Eq.11 reduces to a four-component Hamiltonian, *i.e.*, the substrate potentials  $U_{\ell\ell'}(\mathbf{r})$  are the effective moiré-periodic potentials having moiré-periodicity of their respective moiré interface due to the hBN layer- $\ell' = 1, 4$  on the graphene layers- $\ell = 2, 3$  [4]. The rest of the process of deriving the effective Hamiltonian  $H_{\text{eff}}^{(2)}$  in the main text from 11 is similar to the one described here for the hBN-encapsulated monolayer graphene system. Below, we shall make some more general comments related to such a hBN-BLG-hBN system.

Again, similar to hBN-G-hBN, it contains all the various terms due to the consideration of relaxed graphene sheets in the proximity of the hBN layers. Due to different orientations of the moiré-patterns in each interface, the two potentials are, in general, not commensurate with each other. Owing to the similar geometrical structure to hBN-G-hBN, the two twist angles inherit the same parameter space. Thus, along the line where the two moiré-potentials are commensurate with each other in hBN-G-hBN, here, too, fractality emerges in the relaxed supermoiré structure. To calculate the bandstructure for this system, we first find the relative misorientation using Eq. 9 by which the hBN-layer must be rotated *wrt* the graphene layer such that the moiré-patterns in the two interfaces make a commensurate angle  $\theta_r(q, p)$  between them and then proceed with the calculation of the bandstructure in the main text. Here too the two components  $u_{\parallel}$  and  $\tilde{u}_{\parallel}$  in  $U(\mathbf{r})$  are zero. Within the bandgap of two lowest bands of BLG +  $U_{21}(\mathbf{r})$ , the number of bands that are being inserted due to the presence of  $U_{34}(\mathbf{r})$  again turn out to be  $4(e^{\ln(n_c)/L_N} - 1)$  per spin. In the right panel, we plot the ARPES data in the energy window of the VB of BLG +  $U_{21}(\mathbf{r})$  and the intensity due to the dominant valence band.

### III. GENERIC MODEL HAMILTONIAN FOR MOIRÉ FRACTALS IN STRAINED TWISTED HOMOBILAYERS

For single moiré interfaces in TBLG and G-hBN, the ARPES signal was studied in reference [7] where they used the BM model [8] with equal and different hopping parameters in the local regions AA and AB. Compared to that, the ARPES intensity in this work for a single moiré-interface of TBLG additionally accounts for the strain fields, and the intensity is sensitive to all the hopping parameters in the  $T$ -matrices and the hopping parameters in  $\mathbf{\Lambda}$ -matrices of different  $q$ -shells due to significant changes in the remote valence bands induced by a change in these parameters. To study the electronic effects of atomic relaxations in the MF and model the effect of a substrate as a perturbation to the unrelaxed TBLG via an external periodic potential [9]. In this section, we elucidate the details of such a Hamiltonian for TBLG to underscore their differences compared to the typical BM Hamiltonian.

$$H_j = H_{\text{intra},j}^0 + H_{\text{inter}}^1 \quad (26)$$

where the first term of the Hamiltonian is contributed by the individual layers constituting the system and is termed as intralayer Hamiltonian, which is given by

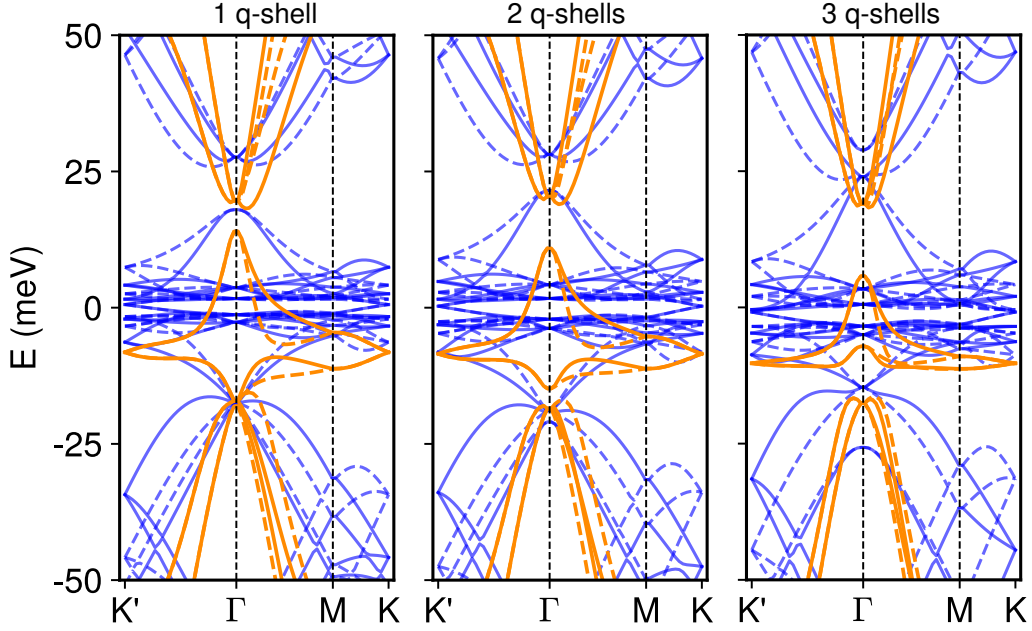

FIG. 1. The band structures for moiré fractals with the (a) 1st shell only, (b) 1st and 2nd shell only and (c) up to 3rd shell for the magic-angle TBLG with  $\theta = 1.05^\circ$  and  $\theta_r(3, 1) = 21.79^\circ$ . The solid lines represent the right valley  $\xi = 1$ , and the dashed lines represent the left valley  $\xi = -1$ . For all shells, the number of bands within the gap of lowest-four bands (with valley degeneracy) remains identically  $4 \left( e^{\ln(n_c)/LN} - 1 \right)$ .

$$H_{\text{intra},j}^0 = \sum_{\ell,\xi} \sum_{S,S'} \int d^2\mathbf{r} \hat{\Psi}_{S,\xi}^{(\ell)\dagger}(\mathbf{r}) \left[ v_F \tilde{\sigma}_{SS'}^{(\ell,\xi)} \cdot \left( \hat{\mathbf{p}} + \gamma \mathcal{A}^{(\ell,\xi)}(\mathbf{r}) \right) + \frac{C_0}{2} (\hat{\mathbf{p}} \cdot \mathcal{A}(\mathbf{r}) + \mathcal{A}(\mathbf{r}) \cdot \hat{\mathbf{p}}) \delta_{SS'} + \right. \\ \left. \beta_1 \left( (\hat{p}_x^2 - \hat{p}_y^2) \sigma_1 + 2\hat{p}_x \hat{p}_y \sigma_2 \right)_{SS'} + \delta_{SS'} V_H(\mathbf{r}) + \delta_{SS'} \sum_{i=1}^j V_i(\mathbf{r}) \right] \hat{\Psi}_{S',\xi}^{(\ell)}(\mathbf{r}) \quad (27)$$

and to the first-order gradients of the fermion fields, the interlayer part of the effective Hamiltonian in Eq.26 is

$$H_{\text{inter}}^1 = \frac{1}{A_{\text{slg}}} \sum_{\xi} \sum_{S,S'} \int d^2\mathbf{r} \left[ T_{SS'}(\mathbf{r}) \hat{\Psi}_S^{(1)\dagger}(\mathbf{r}) \hat{\Psi}_{S'}^{(2)}(\mathbf{r}) + \frac{i}{2} \mathbf{\Lambda}_{SS'}(\mathbf{r}) \cdot \left( \nabla \hat{\Psi}_S^{(1)\dagger}(\mathbf{r}) \hat{\Psi}_{S'}^{(2)}(\mathbf{r}) - \hat{\Psi}_S^{(1)\dagger}(\mathbf{r}) \nabla \hat{\Psi}_{S'}^{(2)}(\mathbf{r}) \right) \right] + \text{h.c.} \quad (28)$$

The term with first-order gradients to fermion fields can be written as

$$\frac{1}{2} \int d^2\mathbf{r} \hat{\Psi}_{S,\xi}^{(1)\dagger}(\mathbf{r}) \{ \hat{\mathbf{p}}, \mathbf{\Lambda}_{SS'}(\mathbf{r}) \} \hat{\Psi}_{S',\xi}^{(2)}(\mathbf{r}) \quad (29)$$

where  $\hat{\mathbf{p}} = -i\hbar\nabla$  is the momentum operator and  $\{..\}$  denotes the anticommutation. The field operator  $\hat{\Psi}_{S,\xi}^{(\ell)}(\mathbf{r})$  is the fermion field operator for sublattice  $S = \text{A,B}$  and valley  $\xi = \pm$  corresponding to the layer- $\ell = t, b$  at a particular location  $\mathbf{r}$ . Here,  $v_F$  is the Fermi velocity [10, 11] in pristine graphene, and  $\mathbf{K}_{\xi}^{(\ell)}$  is the wave vector of the rotated Dirac point of layer- $\ell$  for the valley  $\xi$ . The rotation is accounted by the transformed Pauli matrices  $\tilde{\sigma}^{(\ell,\xi)} = e^{-i\xi\frac{\theta_{\ell}}{2}\sigma_z} (\xi\sigma_x, -\sigma_y) e^{i\xi\frac{\theta_{\ell}}{2}\sigma_z}$ . In the intralayer term of the Hamiltonian (26), we did not consider the terms that are of second-order in the momentum operator as obtained in the model in Ref. [12].

---

[1] Z. Zhu, S. Carr, D. Massatt, M. Luskin, and E. Kaxiras, Twisted trilayer graphene: A precisely tunable platform for correlated electrons, Phys. Rev. Lett. **125**, 116404 (2020).

- [2] P. Moon and M. Koshino, Electronic properties of graphene/hexagonal-boron-nitride moiré superlattice, *Phys. Rev. B* **90**, 155406 (2014).
- [3] E. McCann and V. I. Fal'ko, Landau-level degeneracy and quantum hall effect in a graphite bilayer, *Phys. Rev. Lett.* **96**, 086805 (2006).
- [4] E. McCann and M. Koshino, The electronic properties of bilayer graphene, *Reports on Progress in Physics* **76**, 056503 (2013).
- [5] P. San-Jose, A. Gutiérrez-Rubio, M. Sturla, and F. Guinea, Spontaneous strains and gap in graphene on boron nitride, *Phys. Rev. B* **90**, 075428 (2014).
- [6] P. San-Jose, A. Gutiérrez-Rubio, M. Sturla, and F. Guinea, Electronic structure of spontaneously strained graphene on hexagonal boron nitride, *Phys. Rev. B* **90**, 115152 (2014).
- [7] J. Zhu, J. Shi, and A. H. MacDonald, Theory of angle-resolved photoemission spectroscopy in graphene-based moiré superlattices, *Phys. Rev. B* **103**, 235146 (2021).
- [8] R. Bistritzer and A. H. MacDonald, Moiré bands in twisted double-layer graphene, *Proceedings of the National Academy of Sciences* **108**, 12233 (2011), <https://www.pnas.org/content/108/30/12233.full.pdf>.
- [9] D. Aggarwal, R. Narula, and S. Ghosh, Moiré fractals in twisted graphene layers, *Phys. Rev. B* **109**, 125302 (2024).
- [10] A. H. Castro Neto, F. Guinea, N. M. R. Peres, K. S. Novoselov, and A. K. Geim, The electronic properties of graphene, *Rev. Mod. Phys.* **81**, 109 (2009).
- [11] S. Reich, J. Maultzsch, C. Thomsen, and P. Ordejón, Tight-binding description of graphene, *Phys. Rev. B* **66**, 035412 (2002).
- [12] O. Vafek and J. Kang, Continuum effective hamiltonian for graphene bilayers for an arbitrary smooth lattice deformation from microscopic theories, *Phys. Rev. B* **107**, 075123 (2023).
